# Supplementary material for: Non-Equilibrium Thermodynamics of Harmonically Trapped Bosons
Source: arXiv:1604.03378 source file (2017-06-28)
Supplement: Supplementary file 1 [file Supplementary.pdf]

# Supplementary Material:
# Non-Equilibrium Thermodynamics of Harmonically Trapped Bosons

### Degeneracies in the energy spectrum of the three-atom system

Our aim is to study the dynamics after a quench in the inter- or intra-species coupling constants over a rather large range of values for which three interesting scenarios exist: (i) all the coupling constants are quenched to a non-zero value (i.e. $g_X \in (0, \infty)$ and $g_{XY} \in (0, \infty)$); (ii) only the inter-species coupling constant is quenched and the two X atoms do not interact (i.e. $g_{XY} \in (0, \infty)$ and $g_X = 0$); (iii) the interaction strength between the X atoms is quenched but the Y atom is left non-interacting (i.e. $g_X \in (0, \infty)$ and $g_{XY} = 0$).

The wave-functions in the limit $g \to \infty$ have been thoroughly discussed in the literature [1–3], and we therefore reproduce here just the ansätze which allow to accurately approximate them and which become exact in the infinite limit. They are based on two considerations: 1) when any of the coupling constants tend to infinity the wave function has a zero when the relative coordinate of the atoms that interact vanishes; 2) when the two atoms that interact are the two indistinguishable X atoms the wave function has a definite bosonic symmetry, and therefore the wave function cannot change sign along these zeros. On the contrary, when $g_{XY} \to \infty$, a change of sign along the zeros is not forbidden, as the X and Y atoms are distinguishable.

For the situation $g_{XY} \to \infty$ and $g_X \to \infty$, the wave function has a zero when $x_i - x_j$ or $x_i - y$ equal zero. At the first of these two nodes it cannot change sign, but in the second one the change of sign of the wave function is permitted. An ansatz accounting for these conditions is given by

$$\Psi_1(x_1, x_2, y) \propto e^{-\frac{1}{2}(x_1^2+x_2^2+y^2)}|x_1 - x_2|\ |x_1 - y|\ |x_2 - y|, \tag{1}$$

while the two other possibilities allowing for a change of sign across the $x_i - y$ zero are

$$\Psi_2(x_1, x_2, y) \propto e^{-\frac{1}{2}(x_1^2+x_2^2+y^2)}|x_1 - x_2|(x_1 - y)(x_2 - y), \tag{2}$$

$$\Psi_3(x_1, x_2, y) \propto e^{-\frac{1}{2}(x_1^2+x_2^2+y^2)}|x_1 - x_2| \times [(x_1 - y)\ |x_2 - y| + |x_1 - y|(x_2 - y)]\,. \tag{3}$$

All three wave functions are energetically degenerate for infinite coupling constants. However, for finite but large coupling, the wave function $\Psi_1$ is the ground state, and the highest excited state in this quasi-degenerate triplet is $\Psi_2$. The effect of the different symmetry conditions can also be seen in the energy eigenspectra of the Hamiltonian (26), which we shown in Fig. 8 and Fig. 14 of the main paper. They are numerically calculated using an exact diagonalisation algorithm [4].

More formally, by performing the Jacobi transformation [5, 6]

$$R = \tfrac{1}{3}(x_1 + x_2 + y),\ S = \tfrac{1}{\sqrt{2}}(x_1 - x_2), T = \tfrac{1}{\sqrt{6}}(x_1 + x_2) - \sqrt{\tfrac{3}{2}}y, \tag{4}$$

the Hamiltonian in Eq. (26) can be written as $\mathcal{H} = \mathcal{H}_{\text{com}} + \mathcal{H}_{\text{rel}} + \mathcal{V}_{\text{int}}$, where

$$\begin{aligned} \mathcal{H}_{\text{com}} &= -\frac{1}{2}\left(\partial^2_{R^2} - R^2\right), \quad \mathcal{H}_{\text{rel}} = -\frac{1}{2}\sum_{J=S,T}\left(\partial^2_{J^2} - J^2\right), \\ \mathcal{V}_{\text{int}} &= g_X\delta(S) + g_{XY}\delta(-\frac{1}{2}S + \frac{\sqrt{3}}{2}T) + g_{XY}\delta(-\frac{1}{2}S - \frac{\sqrt{3}}{2}T). \end{aligned} \tag{5}$$

The $\mathcal{H}_{\text{com}}$ part describes the motion of a single atom of mass $M = 3m$ with coordinate $R$ and the relative motion of the three atoms, described by $\mathcal{H}_{\text{rel}}$ and $\mathcal{V}_{\text{int}}$, occurs in the plane defined by variables $S$ and $T$. We consider the computational basis consisting of the eigenstates $|n_R, n_S, n_T\rangle$ of the single-atom Hamiltonian $\mathcal{H}_{\text{sp}} = \mathcal{H}_{\text{com}} + \mathcal{H}_{\text{rel}}$. The COM motion is independent of the relative motion, so that $|n_R, n_S, n_T\rangle = |n_R\rangle \otimes |n_S, n_T\rangle$ with $|n_R\rangle$ being the eigenstates of a one-dimensional harmonic oscillator

$$\psi_{n_R}(R) = \frac{1}{\sqrt[4]{\pi}}\frac{e^{-R^2/2}}{\sqrt{2^{n_R} n_R!}}H_{n_R}(R). \tag{6}$$

For $g_{XY} = g_X = 0$ all wave functions can be written in terms of a basis of Hermite polynomials [7] (see also [8] where an angular basis in the $S - T$ plane is used) and the total energies are given by $E = 3/2 + n_R + n_S + n_T$, where the quantum numbers $n_R$ and $n_T$ can take any integer value. On the contrary $n_S$ is restricted to even values because the wave function has to be even under the interchange of $x_1$ and $x_2$, which is equivalent to the transformation $S \to -S$. The wave functions with the same sum of $n_R + n_S + n_T$ are degenerate, and this explains the degeneracies that occur at vanishing coupling constants in Fig. 8. For $g_{XY} \to \infty = g_X \to \infty$ a triple degeneracy in the ground state appears for large values of the coupling constants, as can be seen

in Fig. 8 quench **A**. The next triplet of excited states corresponds to an excitation of the COM. In the next group some wave functions, which correspond to a second excitation of the COM, overlap with ones which correspond to an excitation of the relative motion (see Ref. [7], where only the REL energies are depicted).

The energy spectrum for three indistinguishable atoms is shown in Fig. 8 quench (∗). In such a case, there is only one coupling constant, $g_{XY} = g_X = g$, and the wave function has to be even when interchanging the Y atom with any of the two X atoms. Thus, for $g = 0$ the wave function also has to be even under this transformation, which spatially corresponds to a reflection with respect to the $S = \pm\sqrt{3}T$ axis (for all possible transformations see Refs. [5, 9]). Note that in this case $n_T$ is no longer a good quantum number even when $g = 0$. For $g \to \infty$ the wave function (1) is the non-degenerate ground state of the system. This is the completely symmetrized version of the Slater determinant which gives the solution for a system of ideal fermions, according to the Bose-Fermi mapping theorem [10, 11]. In this case the functions (2) and (3) are no longer solutions. Note that the three-indistinguishable atom energy spectra show much less degeneracies than in the 2+1 case. Also, as shown in Ref. [7], the ground state for all values of $g_{XY} = g_X$ is exactly the same for both cases.

In the situation where $g_{XY} \to \infty$ and $g_X = 0$, the wave function has to have a zero when $x_i = y$, with no specified symmetry. The ansätze for the two quasi-degenerate lowest energy states are

$$\Psi_1^{(b)}(x_1, x_2, y) \propto e^{-\frac{1}{2}(x_1^2+x_2^2+y^2)}|x_1 - y|\,|x_2 - y|, \tag{7}$$

$$\Psi_3^{(b)}(x_1, x_2, y) \propto e^{-\frac{1}{2}(x_1^2+x_2^2+y^2)}\left[(x_1 - y)\,|x_2 - y| + |x_1 - y|(x_2 - y)\right] \tag{8}$$

and the corresponding energy spectrum is shown in Fig. 8 quench **B**. For very large values of $g_{XY}$ we can observe the double degeneracy of the ground state and the first excited doublet corresponds to an excitation of the COM. On the contrary, the next excited state is a singlet, which has been thoroughly discussed in Refs. [6–8].

The situation where $g_X \to \infty$ and $g_{XY} = 0$, corresponds to a system of a TG gas of 2 atoms in the presence of a non-interacting atom, and the wave function is

$$\Psi_1^{(c)}(x_1, x_2, y) \propto e^{-\frac{1}{2}(x_1^2+x_2^2+y^2)}|x_1 - x_2|. \tag{9}$$

The ground state is non-degenerate and the spectrum as a function of $g_X$ is the sum of the spectra for two atoms, which is analytically solved in [12], and that of a non-interacting third atom (see Fig. 14 quench **C**). Note that the degeneracies present for vanishing coupling constants are lifted in different ways depending on which coupling constant is changed (see Figs. 8 quenches **A** and **B** and Fig. 14 quench **C**).

In the second and third situation the parameters $g_X$ or $g_{XY}$ can be increased towards infinity, and therefore move towards the first situation. The energy spectrum for varying $g_X$ while keeping $g_{XY}$ large is shown in Fig. 14 quench **D** and in this case we can identify states that do not change in energy, which was described as a non-interacting wave function in Refs. [6–8]. Finally, the energy spectrum as a function of $g_{XY}$ and while $g_X$ large is shown in Fig. 14 quench **E**, where non-interacting states can be also identified.

---


[1] M. D. Girardeau, and A. Minguzzi, Phys. Rev. Lett. **99**, 230402 (2007).
[2] F. Deuretzbacher, K. Fredenhagen, D. Becker, K. Bongs, K. Sengstock, and D. Pfannkuche, Phys. Rev. Lett. **100**, 160405 (2008).
[3] J. Levinsen, P. Massignan, G. M. Bruun, and M. M. Parish, Science Advances **1**, e1500197 (2015).
[4] M. A. Garcia-March, and Th. Busch, Phys. Rev. A **87**, 063633 (2013).
[5] N. L. Harshman, Phys. Rev. A **86**, 052122 (2012).
[6] N. T. Zinner, A. G. Volosniev, D. V. Fedorov, A. S. Jensen, and M. Valiente, Europhys. Lett. **107**, 60003 (2014).
[7] M. A. Garcia-March, B. Juliá-Díaz, G.E. Astrakharchik, J. Boronat, and A. Polls, Phys. Rev. A **90**, 063605 (2014).
[8] N. J. S. Loft, A. S. Dehkharghani, N. P. Mehta, A. G. Volosniev, and N. T. Zinner, Eur. Phys. J. D **69**, 65 (2015).
[9] N. L. Harshman, Few-Body Syst., **57**, 11 (2016).
[10] M. Girardeau, J. Math. Phys. **1**, 516 (1960).
[11] M. D. Girardeau, E. M. Wright, and J. M. Triscari, Phys. Rev. A **63**, 033601 (2001).
[12] Th. Busch, B.-G. Englert, K. Rzazewski, and M. Wilkens, Found. Phys. **28**, 549 (1998).
